# Supplementary material for: Fused-Planes: Why Train a Thousand Tri-Planes When You Can Share?
Source: arXiv:2410.23742 source file (2026-02-18)
Supplement: Supplementary file 1 [file msig_costs.tex]

\begin{table}[H]
\footnotesize
\caption{\textbf{Resource costs for MSIG methods with two subsets. } We present the resource costs of MSIG methods that subdivide large sets of scenes into two subsets, as depicted in \cref{eq:total_memory_formula,eq:total_train_time_formula}.
}
\label{tab:msig-costs}
\centering
\vspace{\baselineskip}
\footnotesize
\begin{tabular}{lccccc}
    \toprule

    & $N_1$
    & $\tau_1$ (min)
    & $\tau$ (min)
    & $m_0$ (MB)
    & $\mu$ (MB)\\ \midrule

    CodeNeRF (MSIG)  & 1000 & 14.96 & 9.54 & 3.71   & 0.0026 \\ \midrule
    Fused-Planes-ULW & 500  & 13.72 & 7.16 & 384.19 & 0.0008 \\
    Fused-Planes     & 500  & 14.96 & 8.92 & 360.75 & 0.48 \\

\bottomrule
\end{tabular}
\vskip -0.1in
\end{table}
