# Supplementary material for: Fused-Planes: Why Train a Thousand Tri-Planes When You Can Share?
Source: arXiv:2410.23742 source file (2026-02-18)
Supplement: Supplementary file 2 [file resource_landscape.tex]

\begin{table}[ht]
\caption{\textbf{Resource Costs Comparison.} \karim{TODO update this} This table presents the underlying data behind \cref{fig:general-resource-costs}. Our method showcases the lowest training time and memory costs when training $N = 2000$ scenes, and a comparable NVS quality to Tri-Planes, our base representation. All models are trained on \mbox{$4\times$ NVIDIA L4 GPUs}. \antoine{changer la data sur 1 * L4 + modifier la figure accordingly}} 
\label{tab:resource-costs-landscape-data}
\centering
\vskip 0.15in
\begin{tabular}{lccccc}
\toprule
    & \multicolumn{1}{p{1.8cm}}{\centering Training \\ Time \\ (min $\times 10^3$)} 
    & \multicolumn{1}{p{1.8cm}}{\centering Memory \\ Footprint \\ (MB $\times 10^3$)} 
    & \multicolumn{1}{p{1.8cm}}{\centering \multirow{3}*{PSNR}} \\ \midrule
    Vanilla-NeRF & 318.40 & 25.14 & 40.16  \\ 
    Instant-NGP & 5.50 & 359.40 & 37.71  \\ 
    TensoRF & 34.47 & 397.78 & 40.38  \\ 
    K-Planes & 37.68 & 801.48 & 32.59  \\ \midrule
    Tri-Planes & 32.04 & 3.00 & 30.03 \\
    Ours & 5.22 & 1.08 & 31.20 \\
\bottomrule
\end{tabular}
\vskip -0.1in
\end{table}
